# Supplementary material for: Wiedemann-Franz Law for Molecular Hopping Transport
Source: arXiv:1909.06220 ancillary file (2019-09-13)
Supplement: Supplementary file 1 [file Supplement.pdf]

# Supplemental Material for “Wiedemann-Franz Law for Molecular Hopping Transport”

Galen T. Craven<sup>1</sup> and Abraham Nitzan<sup>1,2</sup>

<sup>1</sup>*Department of Chemistry, University of Pennsylvania, Philadelphia, PA 19104, USA*

<sup>2</sup>*School of Chemistry, Tel Aviv University, Tel Aviv 69978, Israel*

## 1. DERIVATION OF A WIEDEMANN-FRANZ RELATION FOR MOLECULAR SYSTEMS

In this section of the Supplemental Material we present a detailed derivation of a Wiedemann-Franz (WF) relation for purely molecular systems. We define a WF relation as the ratio between a system’s thermal conductivity  $\kappa$  and its electrical conductivity  $\sigma$ .

### A. Electrical Conductivity

Consider a system consisting of identical charge transfer sites at a density  $\rho$  (number of sites per volume) so that the distance between the center of the sites is  $d = \rho^{-1/3}$ . For example, if site density in the system is  $\rho = 10^{21} \text{ cm}^3$  then the distance between centers is 1 nm. The electron transfer (ET) rate between sites over a given distance  $d$  is  $k$ , which is the same in both the forward and backward directions because the sites are identical. Let  $k = k_0 e^{-E_A/k_B T}$  be the hopping rate between sites where  $E_A$  is the activation energy of the reaction,  $T$  is the temperature, and  $k_B$  is the Boltzmann constant. In the presence of an applied electric field  $E$ , the voltage difference between sites in direction of the field is  $V = Ed = E\rho^{-1/3}$ . The number current density (number of electrons moving through a unit area per unit time) is

$$J_n = n_e d k_0 \left( e^{-E_A/k_B T} - e^{-(E_A + eV)/k_B T} \right) \approx \frac{n_e d k_0 e^{-E_A/k_B T} eV}{k_B T} = \frac{n_e d^2 k e E}{k_B T} \quad (\text{S1})$$

$n_e$  is the electron number density. In Eq. (S1),  $d$  multiplies  $k$  because the distance between sites is  $d$  and  $kd$  is speed. We have also used the relation  $V/d = E$ . If  $\rho$  is the site density and  $\chi$  is the number of occupied sites, then

$$n_e = \chi \rho. \quad (\text{S2})$$

The number density is assumed to be low enough relative to number of sites so that Coulomb exclusion does not enter. Note that in the derivation given in the main text we account for

Coulomb exclusion and interparticle correlations, but, as we will show, excluding them does not affect the derived molecular WF relation. Electrical conductivity  $\sigma$  is defined from

$$\mathbf{J}_{\text{el}} = \sigma \frac{V}{d} = \sigma E = e \mathbf{J}_n, \quad (\text{S3})$$

where  $e$  is the electron charge. After using Eq. (S1) we arrive at the result

$$\mathbf{J}_{\text{el}} = \frac{n_e d^2 k_0 e^{-E_A/k_B T} e^2 E}{k_B T} = \frac{n_e d^2 k e^2 E}{k_B T}, \quad (\text{S4})$$

which implies after substitution into Eq. (S3) that the electrical conductivity is

$$\sigma = \frac{n_e d^2 k e^2}{k_B T}. \quad (\text{S5})$$

## B. Thermal Conductivity

Next, consider the same system in the absence of an electric field but in the presence of a temperature gradient. The density of charge transfer sites is again  $\rho$  and the distance between centers is  $d = \rho^{-1/3}$ . The thermal conductivity  $\kappa$  of this system is defined from

$$\mathbf{J}_Q = -\kappa \nabla T, \quad (\text{S6})$$

where  $\mathbf{J}_Q$  is the heat current density and  $\nabla T$  is a temperature gradient. When the temperature gradient is in the  $x$  direction, the heat current density in that same direction is

$$\mathbf{J}_Q = -\kappa \nabla_x T = -\kappa \frac{dT}{dx}. \quad (\text{S7})$$

where  $\nabla_x T = \Delta T/d$ . We want to calculate the thermal conductivity in this system due to electron hopping between sites with different temperatures. To this end, consider two neighboring charge transfer sites  $a$  and  $b$  which have different local temperatures  $T_a = T + \Delta T/2$  and  $T_b = T - \Delta T/2$  but are otherwise identical and thus have the same reorganization energy  $\lambda$  and electron occupation energy  $E'$ . The number of electron hops from site  $a$  to site  $b$  per unit time is  $k\chi$ . Under zero electric current conditions, the same number of hops per unit time occur from site  $b$  to site  $a$ . The heat change in the thermal environment associated with site  $a$  per hop between sites in the  $a \rightarrow b$  and the  $b \rightarrow a$  directions are [1]

$$\mathcal{Q}_{a,b} = \mathcal{Q}_{b,a} = \lambda \left( \frac{T_b - T_a}{T_a + T_b} \right) = -\frac{\lambda}{2} \frac{\Delta T}{T}, \quad (\text{S8})$$

and the heat current (heat transfer per unit time) between sites under steady-state conditions is

$$\mathcal{J}_Q = \chi k (\mathcal{Q}_{a,b} + \mathcal{Q}_{b,a}) = -\frac{\chi k \lambda \Delta T}{T}. \quad (\text{S9})$$

To convert this heat current into a thermal conductivity, consider a volume element with unit surface area and thickness  $d$ . The surface density of sites in this volume element is  $\rho_s = \rho d = d^{-2}$ , which is also a measure of the number of pairs across a surface in a picture where each site on one side of the dividing surface finds its nearest-neighbor on the other side of the surface. The current density in the direction of the temperature gradient is

$$J_Q = \mathcal{J}_Q \rho_s = -\frac{\chi k \lambda \Delta T}{T d^2} = -\frac{\chi k \lambda \nabla_x T}{T d} = -\frac{\chi k \lambda \rho^{1/3} \nabla_x T}{T}, \quad (\text{S10})$$

and after using Eq. (S7) we arrive at

$$\kappa = \frac{\chi k \lambda \rho^{1/3}}{T} = \frac{\chi k \lambda}{T d}, \quad (\text{S11})$$

which is the thermal conductivity due to electron transfer across the temperature gradient  $\nabla T$ .

### C. Molecular Wiedemann-Franz Relation

In metals, the WF law is

$$\frac{\kappa}{\sigma} = \frac{\pi^2}{3} \left( \frac{k_B}{e} \right)^2 T = L_0 T \quad (\text{S12})$$

where  $L_0 = \pi^2/3 (k_B/e)^2$  is the Lorenz number. By combining the results in Eq. (S5) and Eq. (S11) we arrive at the WF relation for molecular systems:

$$\frac{\kappa}{\sigma} = \left( \frac{k_B}{e} \right)^2 \frac{\lambda}{k_B} = L_M T_M \quad (\text{S13})$$

where  $L_M = (k_B/e)^2$  is the Lorenz number for molecular hopping conductance and  $T_M = \lambda/k_B$  is an effective temperature term that is parametrized by the reorganization energy  $\lambda$ .

## 2. WIEDEMANN-FRANZ RELATION IN 1D MOLECULAR SYSTEMS

We now want to derive a WF relation for one-dimensional systems. The pertinent transport properties in one dimension are electrical conductance  $G$  and thermal conductance  $\mathcal{K}$ , and thus the one-dimensional WF relation is given by the ratio  $\mathcal{K}/G$ . Electrical conductance is defined from the relation

$$\mathcal{J}_{\text{el}} = GV, \quad (\text{S14})$$

where  $\mathcal{J}_{\text{el}}$  is an electrical current and  $V$  is a voltage difference. In the presence of an electric field  $E$ , the voltage difference between sites is  $V$  and the electrical current through the chain is

$$\mathcal{J}_{\text{el}} = e \chi k_0 \left( e^{-E_A/k_B T} - e^{-(E_A + eV)/k_B T} \right) = \frac{e \chi k_0 e^{-E_A/k_B T} eV}{k_B T} = \frac{e^2 \chi k V}{k_B T}, \quad (\text{S15})$$

where  $k = k_0 e^{-E_A/k_B T}$ . Equation (S15) is derived in the limit of low electron density where Coulomb repulsion can be ignored. Combining Eqs. (S14) and (S15) we obtain the electrical conductance for this system:

$$G = \frac{e^2 \chi k}{k_B T}. \quad (\text{S16})$$

The thermal conductance is defined from

$$\mathcal{J}_Q = -\mathcal{K} \Delta T, \quad (\text{S17})$$

where  $\mathcal{J}_Q$  is a heat current and  $\Delta T$  is a temperature difference. The heat current between sites in the chain is (see Eq. (S9) and Ref. 1)

$$\mathcal{J}_Q = \chi k (\mathcal{Q}_{a,b} + \mathcal{Q}_{b,a}) = -\frac{\chi k \lambda \Delta T}{T}, \quad (\text{S18})$$

which implies that

$$\mathcal{K} = \frac{\chi k \lambda}{T}. \quad (\text{S19})$$

Thus, for one-dimensional systems, the molecular WF relation  $\mathcal{K}/G$  is the same as in Eq. (S13):

$$\frac{\mathcal{K}}{G} = \left( \frac{k_B}{e} \right)^2 \frac{\lambda}{k_B}. \quad (\text{S20})$$

### 3. WIEDEMANN-FRANZ RELATIONS IN MOLECULAR JUNCTIONS

The system we consider to examine WF relations in molecular junctions consists of a molecular bridge with  $N$  molecular charge transfer sites, labeled  $1, 2, \dots, N$ , which are seated between two metal electrodes that are denoted as  $M_L$  (left) and  $M_R$  (right). Each site  $s$  in the molecular bridge is associated with an electronic occupation energy  $E'_s$  and a set of vibrational modes  $\mathbf{X}_s$  that are in equilibrium with a local thermal environment at temperature  $T_s$ . The coordinate of the  $j$ th vibrational mode is  $x_j$ , the total number of modes in the system is  $v$ , and the total number of modes associated with site  $s$  is  $v_s$ . The left and right electrodes are assumed to be in thermal and electrochemical equilibrium characterized by temperatures  $T_L = T + \Delta T/2$  and  $T_R = T - \Delta T/2$  and chemical potentials  $\mu_L = \mu - \Phi/2$  and  $\mu_R = \mu + \Phi/2$ , respectively, where  $\Delta T = T_L - T_R$  is the temperature bias across the junction,  $T$  is the temperature of the system in the  $\Delta T \rightarrow 0$  limit,  $\mu$  is the Fermi level in the heterogeneous electrodes, and  $\Phi/e = V$  is an applied voltage bias.

In the hopping limit of transport, the electronic motion in the junction is strongly coupled with the vibrational environments about each molecular site and ET proceeds through a hopping

mechanism in which the system has  $N + 1$  electronic states  $a \in \{M, 1, \dots, N\}$  each corresponding to electron localization on either a specific site in the bridge or in the electronic manifold of one of the metals. For example, in state 1 the electron density is localized on molecular site 1, in state 2 the electron density is localized on molecular site 2, and so forth. The special case of  $a = M$  corresponds to the state in which the electron is not found in the junction, that is, in state  $M$  the electron occupies an energy level in one of the metal electrodes.

The response of the vibrational modes to electron localization on each of the molecular sites is described using the Marcus formalism in which the energy in each state is defined by a multidimensional free energy surface:

$$E_a(x_1, x_2, \dots, x_v) = \sum_s^N \sum_{j \in \mathcal{M}^{(s)}} \frac{1}{2} k_j \left( x_j - \bar{x}_j^{(a)} \right)^2 + E'_a, \quad (\text{S21})$$

where  $\bar{x}_j^{(a)}$  is a polaron shift in coordinate  $x_j$  that is induced by electron localization on site  $a$ ,  $k_j$  is the force constant of mode  $j$ ,  $E'_a$  is the electronic energy origin of state  $a$ , and  $\mathcal{M}^{(s)}$  is the set of indices of all modes associated with the  $s$ th site. In the special case of state  $M$ :

$$E_M(x_1, x_2, \dots, x_v) = \sum_s^N \sum_{j \in \mathcal{M}^{(s)}} \frac{1}{2} k_j \left( x_j - \bar{x}_j^{(M)} \right)^2 + \mu. \quad (\text{S22})$$

For a specific state transition  $a \rightarrow b$ , the total reorganization energy of all the modes associated with site  $s$  is

$$\lambda_s^{(a,b)} = \sum_{j \in \mathcal{M}^{(s)}} \frac{1}{2} k_j \left( \bar{x}_j^{(a)} - \bar{x}_j^{(b)} \right)^2, \quad (\text{S23})$$

and the total reorganization energy for the entire vibrational subsystem is

$$\lambda^{(a,b)} = \sum_s^N \sum_{j \in \mathcal{M}^{(s)}} \lambda_j^{(a,b)}. \quad (\text{S24})$$

In the main text, we consider binary hopping between sites which implies that the only modes that are affected by the ET process are those that participate in the particular state transition. In this picture, the total reorganization energy for the transition  $a \rightarrow b$  is

$$\lambda^{(a,b)} = \sum_{s \in \{a,b\}} \lambda_s^{(a,b)}. \quad (\text{S25})$$

Note that in all the numerical calculations shown in the main text we take the reorganization energy of every site to be the same  $\lambda_s^{(a,b)} = \lambda$ .

In the nonadiabatic limit, the ET rate across a thermal gradient between molecular sites is [1]

$$k_{a \rightarrow b} = \frac{|V_{a,b}|^2}{\hbar} \sqrt{\frac{\pi}{k_B (T_a \lambda_a^{(a,b)} + T_b \lambda_b^{(a,b)})}} \exp \left[ -\frac{(\Delta E_{ba} + \lambda^{(a,b)})^2}{4k_B (T_a \lambda_a^{(a,b)} + T_b \lambda_b^{(a,b)})} \right], \quad (\text{S26})$$

where  $V_{a,b}$  is the electronic coupling between states  $a$  and  $b$  and  $\Delta E_{ba} = -\Delta E_{ab} = E'_b - E'_a$  is the reaction free energy. Because of the length scales associated with generating an appreciable temperature gradient between sites, we expect the nonadiabatic limit to be the most pertinent regime for the mechanisms examined in the main text. Equation (S26) is a bithermal (two temperature) variant of the Marcus ET rate; in the unithermal case where  $T_a = T_b = T$ , it reduces to the well-known Marcus ET rate expression that describes phonon-assisted electron hopping between molecular sites under equilibrium conditions.

The ET rates across the thermal gradient between molecule and metal at the left and right electrodes are, respectively [2],

$$k_{1 \rightarrow M_L} = \sqrt{\frac{1}{4\pi k_B T_1 \lambda_1^{(1,M)}}} \int_{\mathbb{R}} [1 - f(T_L, \mu_L, \epsilon)] \Gamma_L(\epsilon) \exp \left[ -\frac{(\Delta E_L + \epsilon + \lambda_1^{(1,M)})^2}{4k_B T_1 \lambda_1^{(1,M)}} \right] d\epsilon, \quad (\text{S27})$$

$$k_{N \rightarrow M_R} = \sqrt{\frac{1}{4\pi k_B T_N \lambda_N^{(N,M)}}} \int_{\mathbb{R}} [1 - f(T_R, \mu_R, \epsilon)] \Gamma_R(\epsilon) \exp \left[ -\frac{(\Delta E_R + \epsilon + \lambda_N^{(N,M)})^2}{4k_B T_N \lambda_N^{(N,M)}} \right] d\epsilon, \quad (\text{S28})$$

and the corresponding rates of electron extraction from metal to molecule are

$$k_{M_L \rightarrow 1} = \sqrt{\frac{1}{4\pi k_B T_1 \lambda_1^{(M,1)}}} \int_{\mathbb{R}} f(T_L, \mu_L, \epsilon) \Gamma_L(\epsilon) \exp \left[ -\frac{(-\Delta E_L - \epsilon + \lambda_1^{(M,1)})^2}{4k_B T_1 \lambda_1^{(M,1)}} \right] d\epsilon, \quad (\text{S29})$$

$$k_{M_R \rightarrow N} = \sqrt{\frac{1}{4\pi k_B T_N \lambda_N^{(M,N)}}} \int_{\mathbb{R}} f(T_R, \mu_R, \epsilon) \Gamma_R(\epsilon) \exp \left[ -\frac{(-\Delta E_R - \epsilon + \lambda_N^{(M,N)})^2}{4k_B T_N \lambda_N^{(M,N)}} \right] d\epsilon, \quad (\text{S30})$$

where  $f(T, \mu, \epsilon) = (\exp[(\epsilon - \mu)/k_B T] + 1)^{-1}$  is the Fermi-Dirac distribution and

$$\Gamma_E(\epsilon) = \left( \frac{2\pi}{\hbar} |V_E|^2 \rho_E \right)_\epsilon : E \in \{L, R\}, \quad (\text{S31})$$

defines the molecule-metal coupling strength at the corresponding electrode. The single electron density of states  $\rho_E$  and the tunneling coupling for electron transfer between molecule and metal  $V_E$  both formally depend on the energy level  $\epsilon$ . This explicit energy dependence is shown in all analytical derivations, however, in the numerical calculations shown in the main text, the wide-band approximation is applied, and thus  $\Gamma_L$  and  $\Gamma_R$  are taken as constants. The reaction free energy for the state transition  $1 \rightarrow M$  is

$$\Delta E_L = E'_M - E'_1, \quad (\text{S32})$$

and for the  $N \rightarrow M$  transition

$$\Delta E_R = E'_M - E'_N. \quad (\text{S33})$$

In the standard unithermal limit, the results in Eqs. (S27) - (S30) reduce to the traditional Marcus-Hush-Chidsey rate expressions for equilibrium heterogeneous ET [3–8].

The electronic current in the junction  $\mathcal{J}_{\text{el}}$  can be derived in the electron hopping regime from the kinetic master equations describing the probability to observe the system in each electronic state, where each state corresponds to the localization of electron density on a specific site in the bridge or in one of the electrodes. The probability that the system is in state  $a \in \{M, 1, \dots, N\}$  is  $\mathcal{P}_a$  with  $\mathcal{P}_M$  being the probability that the electron occupies an energy level in the electronic manifold of one of the electrodes. The kinetic equations describing the probabilities to observe the system in each of the  $N + 1$  electronic states are

$$\begin{aligned} \dot{\mathcal{P}}_M &= -k_{M_L \rightarrow 1} \mathcal{P}_M + k_{1 \rightarrow M_L} \mathcal{P}_1 - k_{M_R \rightarrow N} \mathcal{P}_M + k_{N \rightarrow M_R} \mathcal{P}_N, \\ \dot{\mathcal{P}}_1 &= -(k_{1 \rightarrow M_L} + k_{1 \rightarrow 2}) \mathcal{P}_1 + k_{M_L \rightarrow 1} \mathcal{P}_M + k_{2 \rightarrow 1} \mathcal{P}_2, \\ &\dots \\ \dot{\mathcal{P}}_a &= -(k_{a \rightarrow a+1} + k_{a \rightarrow a-1}) \mathcal{P}_a + k_{a+1 \rightarrow a} \mathcal{P}_{a+1} + k_{a-1 \rightarrow a} \mathcal{P}_{a-1}, \\ &\dots \\ \dot{\mathcal{P}}_{N-1} &= -(k_{N-1 \rightarrow N} + k_{N-1 \rightarrow N-2}) \mathcal{P}_{N-1} + k_{N \rightarrow N-1} \mathcal{P}_N + k_{N-2 \rightarrow N-1} \mathcal{P}_{N-2}, \\ \dot{\mathcal{P}}_N &= -(k_{N \rightarrow M_R} + k_{N \rightarrow N-1}) \mathcal{P}_N + k_{M_R \rightarrow N} \mathcal{P}_M + k_{N-1 \rightarrow N} \mathcal{P}_{N-1}. \end{aligned} \quad (\text{S34})$$

At steady state (ss),  $\dot{\mathcal{P}}_a = 0 \forall a$  which transforms the set of differential equations (S34) into a set of algebraic equations which can be written as

$$\mathbf{K} \mathbf{P}^{(\text{ss})} = \mathbf{S} \quad (\text{S35})$$

where  $\mathbf{P}^{(\text{ss})} = \{\mathcal{P}_M^{(\text{ss})}, \mathcal{P}_1^{(\text{ss})}, \dots, \mathcal{P}_N^{(\text{ss})}\}$  is a set of occupancy probabilities for each electronic state under steady-state conditions,  $\mathbf{K}$  is the matrix of rate coefficients describing the RHS of the system of equations (S34), and  $\mathbf{S}$  is a column of constants. This system of algebraic equations is singular, however, it can be solved by augmenting the system with the probability conservation equation

$$\mathcal{P}_M + \sum_{j=1}^N \mathcal{P}_j = 1. \quad (\text{S36})$$

The solution of Eq. (S35) is

$$\mathbf{P}^{(\text{ss})} = \mathbf{K}^{-1} \mathbf{S}, \quad (\text{S37})$$

where  $\mathbf{K}^{-1}$  is the inverse of  $\mathbf{K}$ . The occupancy probabilities from (S37) can be used to obtain the steady-state electronic current:

$$\frac{\mathcal{J}_{\text{el}}}{e} = -k_{\text{M}_L \rightarrow 1} \mathcal{P}_{\text{M}}^{(\text{ss})} + k_{1 \rightarrow \text{M}_L} \mathcal{P}_1^{(\text{ss})}. \quad (\text{S38})$$

Electron transfer across the thermal gradient in the molecular junction generates a heat current at both molecule-metal interfaces and either into or out of the thermal environment of each molecular site. For binary molecule-to-molecule ET in the bridge, the heat change in the thermal environment of site  $s$  during each state transition  $a \rightarrow b$  is

$$\mathcal{Q}_{a,b}^{(s)} = \frac{T_s \lambda_s^{(a,b)} (E'_a - E'_b) + \sum_{\substack{\alpha \in \{a,b\} \\ \alpha \neq s}} (T_\alpha - T_s) \lambda_a^{(a,b)} \lambda_b^{(a,b)}}{T_a \lambda_a^{(a,b)} + T_b \lambda_b^{(a,b)}}. \quad (\text{S39})$$

The ETI heat current  $\mathcal{J}_Q^{(s)}$  associated with site  $s$  is a product of heat change per electron terms  $\mathcal{Q}_{a,b}^{(s)}$  and unidirectional electronic flux terms of the form  $k_{a \rightarrow b} \mathcal{P}_a$ , taken over all state transitions that affect that site. Specifically, the system of equations that expresses the ETI heat current associated with the environment of each molecular site is

$$\begin{aligned} \mathcal{J}_Q^{(1)} &= -\mathcal{J}_Q^{(\text{L})} + k_{1 \rightarrow 2} \mathcal{P}_1 \mathcal{Q}_{1,2}^{(1)} + k_{2 \rightarrow 1} \mathcal{P}_2 \mathcal{Q}_{2,1}^{(1)}, \\ \mathcal{J}_Q^{(2)} &= k_{1 \rightarrow 2} \mathcal{P}_1 \mathcal{Q}_{1,2}^{(2)} + k_{2 \rightarrow 1} \mathcal{P}_2 \mathcal{Q}_{2,1}^{(2)} + k_{2 \rightarrow 3} \mathcal{P}_2 \mathcal{Q}_{2,3}^{(2)} + k_{3 \rightarrow 2} \mathcal{P}_3 \mathcal{Q}_{3,2}^{(2)}, \\ &\dots \\ \mathcal{J}_Q^{(s)} &= k_{s-1 \rightarrow s} \mathcal{P}_{s-1} \mathcal{Q}_{s-1,s}^{(s)} + k_{s \rightarrow s-1} \mathcal{P}_s \mathcal{Q}_{s,s-1}^{(s)} \\ &\quad + k_{s \rightarrow s+1} \mathcal{P}_s \mathcal{Q}_{s,s+1}^{(s)} + k_{s+1 \rightarrow s} \mathcal{P}_{s+1} \mathcal{Q}_{s+1,s}^{(s)}, \\ &\dots \\ \mathcal{J}_Q^{(N-1)} &= k_{N-2 \rightarrow N-1} \mathcal{P}_{N-2} \mathcal{Q}_{N-2,N-1}^{(N-1)} + k_{N-1 \rightarrow N-2} \mathcal{P}_{N-1} \mathcal{Q}_{N-1,N-2}^{(N-1)} \\ &\quad + k_{N-1 \rightarrow N} \mathcal{P}_{N-1} \mathcal{Q}_{N-1,N}^{(N-1)} + k_{N \rightarrow N-1} \mathcal{P}_N \mathcal{Q}_{N,N-1}^{(N-1)}, \\ \mathcal{J}_Q^{(N)} &= -\mathcal{J}_Q^{(\text{R})} + k_{N-1 \rightarrow N} \mathcal{P}_{N-1} \mathcal{Q}_{N-1,N}^{(N)} + k_{N \rightarrow N-1} \mathcal{P}_N \mathcal{Q}_{N,N-1}^{(N)}, \end{aligned} \quad (\text{S40})$$

where  $\mathcal{J}_Q^{(\text{L})}$  and  $\mathcal{J}_Q^{(\text{R})}$  are the ETI heat currents at the left and right electrodes. The ETI heat current between molecule and metal at the left electrode is

$$\begin{aligned} \mathcal{J}_Q^{(\text{L})} &= \int_{\mathbb{R}^{|X_1|}} \mathcal{P}_1 [1 - f(T_L, \mu_L, E_L(\mathbf{X}_1))] \Gamma(E_L(\mathbf{X}_1)) \\ &\quad \times (E_L(\mathbf{X}_1) - \mu_L) \frac{\exp[-E_{1,1}^\dagger(\mathbf{X}_1)/k_B T_1]}{Z_{1,1}^\dagger} d\mathbf{X}_1 \\ &\quad + \int_{\mathbb{R}^{|X_1|}} \mathcal{P}_M f(T_L, \mu_L, E_L(\mathbf{X}_1)) \Gamma(E_L(\mathbf{X}_1)) \\ &\quad \times (\mu_L - E_L(\mathbf{X}_1)) \frac{\exp[-E_{M,1}^\dagger(\mathbf{X}_1)/k_B T_1]}{Z_{M,1}^\dagger} d\mathbf{X}_1, \end{aligned} \quad (\text{S41})$$

and at the right electrode

$$\begin{aligned}
\mathcal{J}_Q^{(R)} = & \int_{\mathbb{R}^{|\mathbf{x}_N|}} \mathcal{P}_N [1 - f(T_R, \mu_R, E_R(\mathbf{X}_N))] \Gamma_R(E_R(\mathbf{X}_N)) \\
& \times (E_R(\mathbf{X}_N) - \mu_R) \frac{\exp[-E_{N,N}^\dagger(\mathbf{X}_N)/k_B T_N]}{Z_{N,N}^\dagger} d\mathbf{X}_N \\
& + \int_{\mathbb{R}^{|\mathbf{x}_N|}} \mathcal{P}_M f(T_R, \mu_R, E_R(\mathbf{X}_N)) \Gamma_R(E_R(\mathbf{X}_N)) \\
& \times (\mu_R - E_R(\mathbf{X}_N)) \frac{\exp[-E_{M,N}^\dagger(\mathbf{X}_N)/k_B T_N]}{Z_{M,N}^\dagger} d\mathbf{X}_N,
\end{aligned} \tag{S42}$$

where

$$E_L(\mathbf{X}_1) = -\Delta E_R + \sum_{j \in \mathcal{M}^{(1)}} k_j (\bar{x}_j^{(M)} - \bar{x}_j^{(1)}) x_j + \frac{1}{2} k_j (\bar{x}_j^{(1)})^2 - \frac{1}{2} k_j (\bar{x}_j^{(M)})^2 \tag{S43}$$

is the the energy difference between surfaces  $E_1$  and  $E_M$  taken over all the modes associated with site 1,

$$E_R(\mathbf{X}_N) = -\Delta E_L + \sum_{j \in \mathcal{M}^{(N)}} k_j (\bar{x}_j^{(M)} - \bar{x}_j^{(N)}) x_j + \frac{1}{2} k_j (\bar{x}_j^{(N)})^2 - \frac{1}{2} k_j (\bar{x}_j^{(M)})^2 \tag{S44}$$

is energy difference between surfaces  $E_N$  and  $E_M$  taken over all the modes associated with site  $N$ ,

$$E_{a,s}^\dagger(\mathbf{X}_s) = \sum_{j \in \mathcal{M}^{(s)}} \frac{1}{2} k_j (x_j - \bar{x}_j^{(a)})^2 \tag{S45}$$

denotes the energy of above the corresponding energy origin  $E'_a$  in state  $a$  taken over all of the modes associated with site  $s$ , and

$$Z_{a,s}^\dagger = \int_{\mathbb{R}^{|\mathbf{x}_s|}} \exp[-E_{a,s}^\dagger(\mathbf{X}_s)/k_B T_s] d\mathbf{X}_s = \prod_{j \in \mathcal{M}^{(s)}} \sqrt{\frac{2\pi k_B T_s}{k_j}} \tag{S46}$$

is a configuration integral. In Eqs. (S41), (S42), and (S46),  $|\mathbf{X}_s|$  is the number of modes associated with site  $s$  and  $d\mathbf{X}_s = \prod_{j \in \mathcal{M}^{(s)}} dx_j$  is a differential volume element. The steady-state limit of the heat currents in Eqs. (S40)-(S42) are obtained by replacing all  $\mathcal{P}$  terms with the corresponding  $\mathcal{P}^{(ss)}$  terms.

The temperature profile in the molecular bridge is defined through application of a self-consistent reservoir (SCR) method that is adapted to treat ETIHT. Specifically, the bridge temperatures  $T_1, T_2, \dots, T_N$  and the potential bias  $\Phi$  are defined subject to the constraints:

$$\mathcal{J}_Q^{(s)} = 0 \forall s \in \{1, 2, \dots, N\} \quad \text{and} \quad \mathcal{J}_{el} = 0, \tag{S47}$$

which state that we require the heat currents associated with all molecular sites and also the electronic current through the junction to vanish. These conditions ensure that a non-zero net

heat current exists only at the two molecule-metal interfaces. The root-finding procedure used to satisfy (S47) is performed using a multidimensional Newton-Raphson method. Note that the heat current terms are highly nonlinear in  $T_1, T_2, \dots, T_N$  and  $\Phi$ , and thus the root-finding operation can be complex.

After the temperature profile and voltage bias are obtained using the modified SCR method, the heat current at the hot electrode is equal in magnitude but opposite in sign to the heat current at the cold electrode:

$$\mathcal{J}_{\mathcal{Q}}^{(\text{L})} = -\mathcal{J}_{\mathcal{Q}}^{(\text{R})}, \quad (\text{S48})$$

and the the ETI heat current is

$$\mathcal{J}_{\mathcal{Q}} = |\mathcal{J}_{\mathcal{Q}}^{(\text{L})}| = |\mathcal{J}_{\mathcal{Q}}^{(\text{R})}|. \quad (\text{S49})$$

The ETI thermal conductance is defined as

$$\mathcal{K} = \lim_{\Delta T \rightarrow 0} \left. \frac{\mathcal{J}_{\mathcal{Q}}}{\Delta T} \right|_{\mathcal{J}_{\text{el}}=0}. \quad (\text{S50})$$

The corresponding electrical conductance is

$$G = \lim_{\Phi \rightarrow 0} \left. \frac{e\mathcal{J}_{\text{el}}}{\Phi} \right|_{\Delta T=0}, \quad (\text{S51})$$

where  $\mathcal{J}_{\text{el}}$  is taken from Eq. (S38). The conductance ratios  $\mathcal{K}/G$  shown in the main text are calculated in the linear response regime. The thermal conductance values are measured by calculating the heat current at a specific temperature  $T$  under zero electrical current conditions for  $\Delta T = \Delta T_+ = 1$  K and  $\Delta T = \Delta T_- = -1$  K and then obtaining the thermal conductance as

$$\mathcal{K} = \frac{\mathcal{J}_{\mathcal{Q}}(\Delta T_+) - \mathcal{J}_{\mathcal{Q}}(\Delta T_-)}{\Delta T_+ - \Delta T_-}. \quad (\text{S52})$$

The electrical conductance values are measured in a similar fashion by calculating the electric current at a specific temperature  $T$  with no temperature bias  $\Delta T = 0$  for  $\Phi = \Phi_+ = 0.005$  eV and  $\Phi = \Phi_- = -0.005$  eV and then obtaining the electrical conductance as

$$G = \frac{\mathcal{J}_{\text{el}}(\Phi_+) - \mathcal{J}_{\text{el}}(\Phi_-)}{\Phi_+ - \Phi_-}. \quad (\text{S53})$$

#### 4. BALLISTIC ELECTRON TRANSPORT IN A MOLECULAR JUNCTION

In the ballistic limit of transport, the electronic motion through the junction described in Section 3 is decoupled from the vibrational thermal environments about each site in the molecular

bridge. Therefore, the electronic current, heat current, and electronic thermal conductance are independent of the local temperatures in the bridge  $T_1, T_2, \dots, T_N$  and the reorganization energies  $\lambda_s$ . The electronic current in the ballistic limit can be expressed using the Landauer form [9]

$$\frac{\mathcal{J}_{\text{el}}}{e} = \frac{1}{\pi\hbar} \int_{-\infty}^{\infty} \mathcal{T}(\epsilon) \left[ f(T_{\text{R}}, \mu_{\text{R}}, \epsilon) - f(T_{\text{L}}, \mu_{\text{L}}, \epsilon) \right] d\epsilon, \quad (\text{S54})$$

where  $\mathcal{T}(\epsilon)$  is the electronic transmission function calculated using a nonequilibrium Green's function (NEGF) approach with

$$\mathcal{T}(\epsilon) = \text{Tr} \left[ \hat{\Gamma}_{\text{L}}(\epsilon) \hat{G}^{\dagger}(\epsilon) \hat{\Gamma}_{\text{R}}(\epsilon) \hat{G}(\epsilon) \right], \quad (\text{S55})$$

where the bridge Green's function  $\hat{G}$  (with conjugate adjoint  $\hat{G}^{\dagger}$ ) satisfies

$$\hat{G}^{-1}(\epsilon) = \begin{pmatrix} \epsilon - E'_1 + \frac{1}{2}i\hbar\Gamma_{\text{L}}(\epsilon) & V_{1,2} & 0 & 0 & \dots & 0 \\ V_{2,1} & \epsilon - E'_2 & V_{2,3} & 0 & \dots & 0 \\ 0 & V_{3,2} & \epsilon - E'_3 & V_{3,4} & & \vdots \\ 0 & 0 & V_{4,3} & \ddots & \ddots & 0 \\ \vdots & \vdots & & \ddots & \epsilon - E'_{N-1} & V_{N-1,N} \\ 0 & 0 & \dots & 0 & V_{N,N-1} & \epsilon - E'_N + \frac{1}{2}i\hbar\Gamma_{\text{R}}(\epsilon) \end{pmatrix}, \quad (\text{S56})$$

with

$$\hat{\Gamma}_{\text{L}}(\epsilon) = \begin{pmatrix} \hbar\Gamma_{\text{L}}(\epsilon) & 0 & \dots & 0 \\ 0 & 0 & \dots & 0 \\ \vdots & \vdots & \ddots & \vdots \\ 0 & 0 & \dots & 0 \end{pmatrix}, \quad (\text{S57})$$

and

$$\hat{\Gamma}_{\text{R}}(\epsilon) = \begin{pmatrix} 0 & 0 & \dots & 0 \\ 0 & 0 & \dots & 0 \\ \vdots & \vdots & \ddots & \vdots \\ 0 & 0 & \dots & \hbar\Gamma_{\text{R}}(\epsilon) \end{pmatrix}, \quad (\text{S58})$$

being the molecule-metal coupling matrices. Note that the wide-band approximation is applied in all numerical calculations in the main text which implies that  $\Gamma_{\text{L}}$  and  $\Gamma_{\text{R}}$  are constants. The heat current generated by electron transport across the junction is

$$\mathcal{J}_{\text{Q}} = \frac{1}{\pi\hbar} \int_{-\infty}^{\infty} \mathcal{T}(\epsilon) (\epsilon - \mu) \left[ f(T_{\text{R}}, \mu_{\text{R}}, \epsilon) - f(T_{\text{L}}, \mu_{\text{L}}, \epsilon) \right] d\epsilon, \quad (\text{S59})$$

which is evaluated under the condition of zero electronic current  $\mathcal{J}_Q|_{\mathcal{J}_{\text{el}}=0}$ . The zero electronic current condition is enforced through variation of the potential bias  $\Phi$ . The electronic thermal conductance is defined as

$$\mathcal{K} = \lim_{\Delta T \rightarrow 0} \left. \frac{\mathcal{J}_Q}{\Delta T} \right|_{\mathcal{J}_{\text{el}}=0}, \quad (\text{S60})$$

and the electrical conductance is

$$G = \lim_{\Phi \rightarrow 0} \left. \frac{e\mathcal{J}_{\text{el}}}{\Phi} \right|_{\Delta T=0} \quad (\text{S61})$$

where  $\mathcal{J}_{\text{el}}$  is taken from Eq. (S54). The ballistic conductance ratios  $\mathcal{K}/G$  shown in the main text are calculated in the linear response regime using the same procedure applied in the hopping case (See Section 3).

## 5. SUPPLEMENTARY CONDUCTANCE RATIO CALCULATIONS

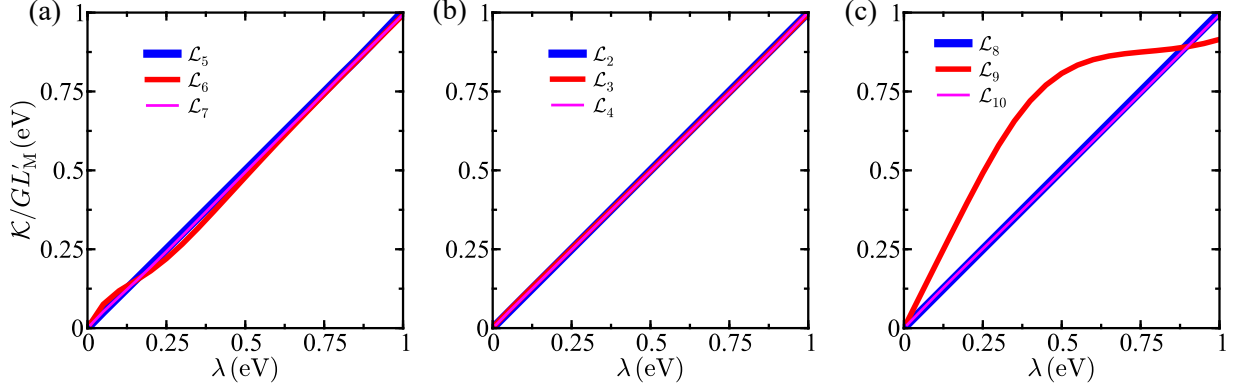

FIG. S1. Calculated conductance ratio  $\mathcal{K}/GL'_M$  with  $L'_M = L_M/k_B$  as a function of reorganization energy  $\lambda$  in a model molecular junction with  $N = 5$  sites. We denote the energy landscape defined by a linear ramp of energy levels from energy  $E'_1$  to energy  $E'_N$  as  $[E'_1, E'_N]$ . (a) Conductance ratios at 300 K for energy landscapes  $\mathcal{L}_5 \equiv [0.3 \text{ eV}, 0]$  (blue),  $\mathcal{L}_6 \equiv [-0.1 \text{ eV}, -0.4 \text{ eV}]$  (red), and  $\mathcal{L}_7 \equiv [0, -0.3 \text{ eV}]$  (magenta). Notice that the magenta line aligns over the blue line. (b) Conductance ratios at 1000 K for energy landscapes  $\mathcal{L}_2 \equiv E'_s = 0.25 \text{ eV} \forall s$  (blue),  $\mathcal{L}_3 \equiv E'_s = -0.25 \text{ eV} \forall s$  (red), and  $\mathcal{L}_4 \equiv [0.15 \text{ eV}, -0.15 \text{ eV}]$  (magenta). Note that all of the lines are aligned. (c) Conductance ratios at 1000 K for energy landscapes  $\mathcal{L}_8 \equiv E'_s = 1 \text{ eV} \forall s$  (blue),  $\mathcal{L}_9 \equiv -1 \text{ eV} \forall s$  (red), and  $\mathcal{L}_{10} \equiv [-1 \text{ eV}, 0]$  (magenta). The magenta line aligns over the blue line. In all calculations shown in this Figure, the electronic coupling between molecular sites is 0.01 eV and the tunneling coupling for ET between molecule and metal is  $\approx 0.07 \text{ eV}$ .

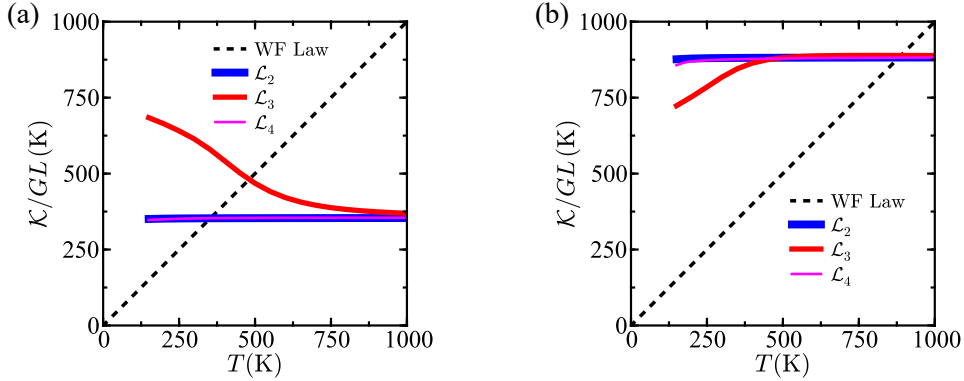

FIG. S2. The calculated conductance ratio  $\mathcal{K}/GL$  as a function of temperature  $T$  in a model molecular junction with  $N = 5$  sites. The results are shown for energy landscapes  $\mathcal{L}_2 \equiv E'_s = 0.25 \text{ eV} \forall s$  (blue),  $\mathcal{L}_3 \equiv E'_s = -0.25 \text{ eV} \forall s$  (red), and  $\mathcal{L}_4 \equiv [0.15 \text{ eV}, -0.15 \text{ eV}]$  (magenta) with (a)  $\lambda = 0.1 \text{ eV}$  and (b)  $\lambda = 0.25 \text{ eV}$ . The black dashed diagonal line in each panel is the result predicted by the WF law. In all calculations shown in this Figure, the electronic coupling between molecular sites is 0.01 eV and the tunneling coupling for ET between molecule and metal is  $\approx 0.07 \text{ eV}$ .

- 
- [1] G. T. Craven and A. Nitzan, Proc. Natl. Acad. Sci. **113**, 9421 (2016), doi:10.1073/pnas.1609141113.
  - [2] G. T. Craven and A. Nitzan, J. Chem. Phys. **146**, 092305 (2017), doi:10.1063/1.4971293.
  - [3] R. A. Marcus, J. Chem. Phys. **43**, 679 (1965), doi:10.1063/1.1696792.
  - [4] N. Hush, Electrochim. Acta **13**, 1005 (1968), doi:10.1016/0013-4686(68)80032-5.
  - [5] C. E. D. Chidsey, Science **251**, 919 (1991), doi:10.1126/science.251.4996.919.
  - [6] A. Nitzan, *Chemical Dynamics in Condensed Phases: Relaxation, Transfer, and Reactions in Condensed Molecular Systems* (Oxford University Press, 2006).
  - [7] A. Migliore and A. Nitzan, ACS Nano **5**, 6669 (2011), doi:10.1021/nn202206e.
  - [8] E. Laborda, M. C. Henstridge, and R. G. Compton, J. Electroanal. Chem. **667**, 48 (2012), ISSN 1572-6657, doi:10.1016/j.jelechem.2011.12.011.
  - [9] M. Galperin, A. Nitzan, and M. A. Ratner, Mol. Phys. **106**, 397 (2008), doi:10.1080/00268970701837784.
